# Supplementary material for: PRD: Peer Rank and Discussion Improve Large Language Model based Evaluations
Source: arXiv:2307.02762 source file (2024-12-31)
Supplement: Supplementary file 1 [file additional_elo_results.tex]

% \onecolumn
\section{Additional LLMs Elo Results}
\label{sec:additional_results}

% Please add the following required packages to your document preamble:
% \usepackage{graphicx}
\begin{table}[h]
\centering
\resizebox{0.55\columnwidth}{!}{%
\begin{tabular}{l|llll|ll}
\toprule
& \multicolumn{2}{c}{All} & \multicolumn{2}{c}{All (Weighted)} & \multicolumn{2}{|c}{Human Raters} \\
        \cmidrule(lr){2-3} \cmidrule(lr){4-5} \cmidrule(lr){6-7}
models  & Elo & Rank & Elo & Rank & Elo & Rank \\
\midrule
Vicuna    & 999  & 2    & 1011 (-47)     & 1         & 1058         & 1    \\
Zephyr    & 1010 & 1    & 1007 (+7)      & 2         & 1000         & 2    \\
GPT-3.5   & 991  & 3    & 993 (+52)      & 3         & 941          & 3    \\
\bottomrule
\end{tabular}%
}
\caption{Additional Elo Scores}
\label{tab:additional_results}
\end{table}

In Table \ref{tab:additional_results}, we present the results on GPT-3.5 and emerging LLMs Vicuna-13b/7b, and Zephyr-7b-alpha. We show that the ranking and Elo scores under our approach are closer to golden results (consistent with results in the main paper). This change demonstrates that our PR method is important and has a better alignment with human judgment.
